# Supplementary material for: Neural operator learning of heterogeneous mechanobiological insults contributing to aortic aneurysms
Source: arXiv:2205.03780 source file (2022-05-08)
Supplement: Supplementary file 1 [file D-additional.tex]

\section{Additional results}
\label{app:appendix_d}

\subsection{Insult type}

\noindent Predicting insult profiles with information at $5 \times 5$ sensor locations is sufficiently accurate for cases with $\theta_{od} < 260^\circ$ and relatively small $z_{od}$. However, with a wider $\theta_{od}$ and broader $z_{od}$, limited information within a single-spaced neighborhood around maximum dilatation and minimum distensibility is insufficient; hence, for such cases, the relative error increases. Because a wider region is captured in the 9 double-spaced sensor placement, the prediction improves. Finally, the full-field CNN-based architecture achieves the best prediction.

% --------------------------------
\begin{figure}[!htbp]
\centering
\includegraphics[width=0.9\textwidth]{figures/ax-circ-width.png}
\caption{Pending.}
\label{fig:ax-circ-width}
\end{figure}
% --------------------------------

\subsection{Insult region size}

% % --------------------------------
% \begin{figure}[!htbp]
% \centering
% \includegraphics[width=\textwidth]{figures/}
% \caption{}
% \label{}
% \end{figure}
% % --------------------------------

\subsection{Normotensive and hypertensive conditions}

% % --------------------------------
% \begin{figure}[!htbp]
% \centering
% \includegraphics[width=\textwidth]{figures/}
% \caption{}
% \label{}
% \end{figure}
% % --------------------------------
